# Supplementary material for: Engineering vibrationally-assisted energy transfer in a trapped-ion quantum simulator
Source: arXiv:1709.04064 source file (2018-04-06)
Supplement: Supplementary file 1 [file supplfig.tex]

%auto-ignore
\documentclass{standalone}
\usepackage{tikz}
\usetikzlibrary{decorations.pathmorphing}
\usetikzlibrary{decorations.markings}
\usetikzlibrary{arrows,decorations}
\usetikzlibrary{shapes.misc, positioning}
\usetikzlibrary{shapes.arrows, fadings, calc}

\begin{document}
\begin{tikzpicture}[scale = 1.0]
\node[inner sep=0pt] (trap) at (-1.0,  0.0) {\includegraphics[width=0.45\textwidth]{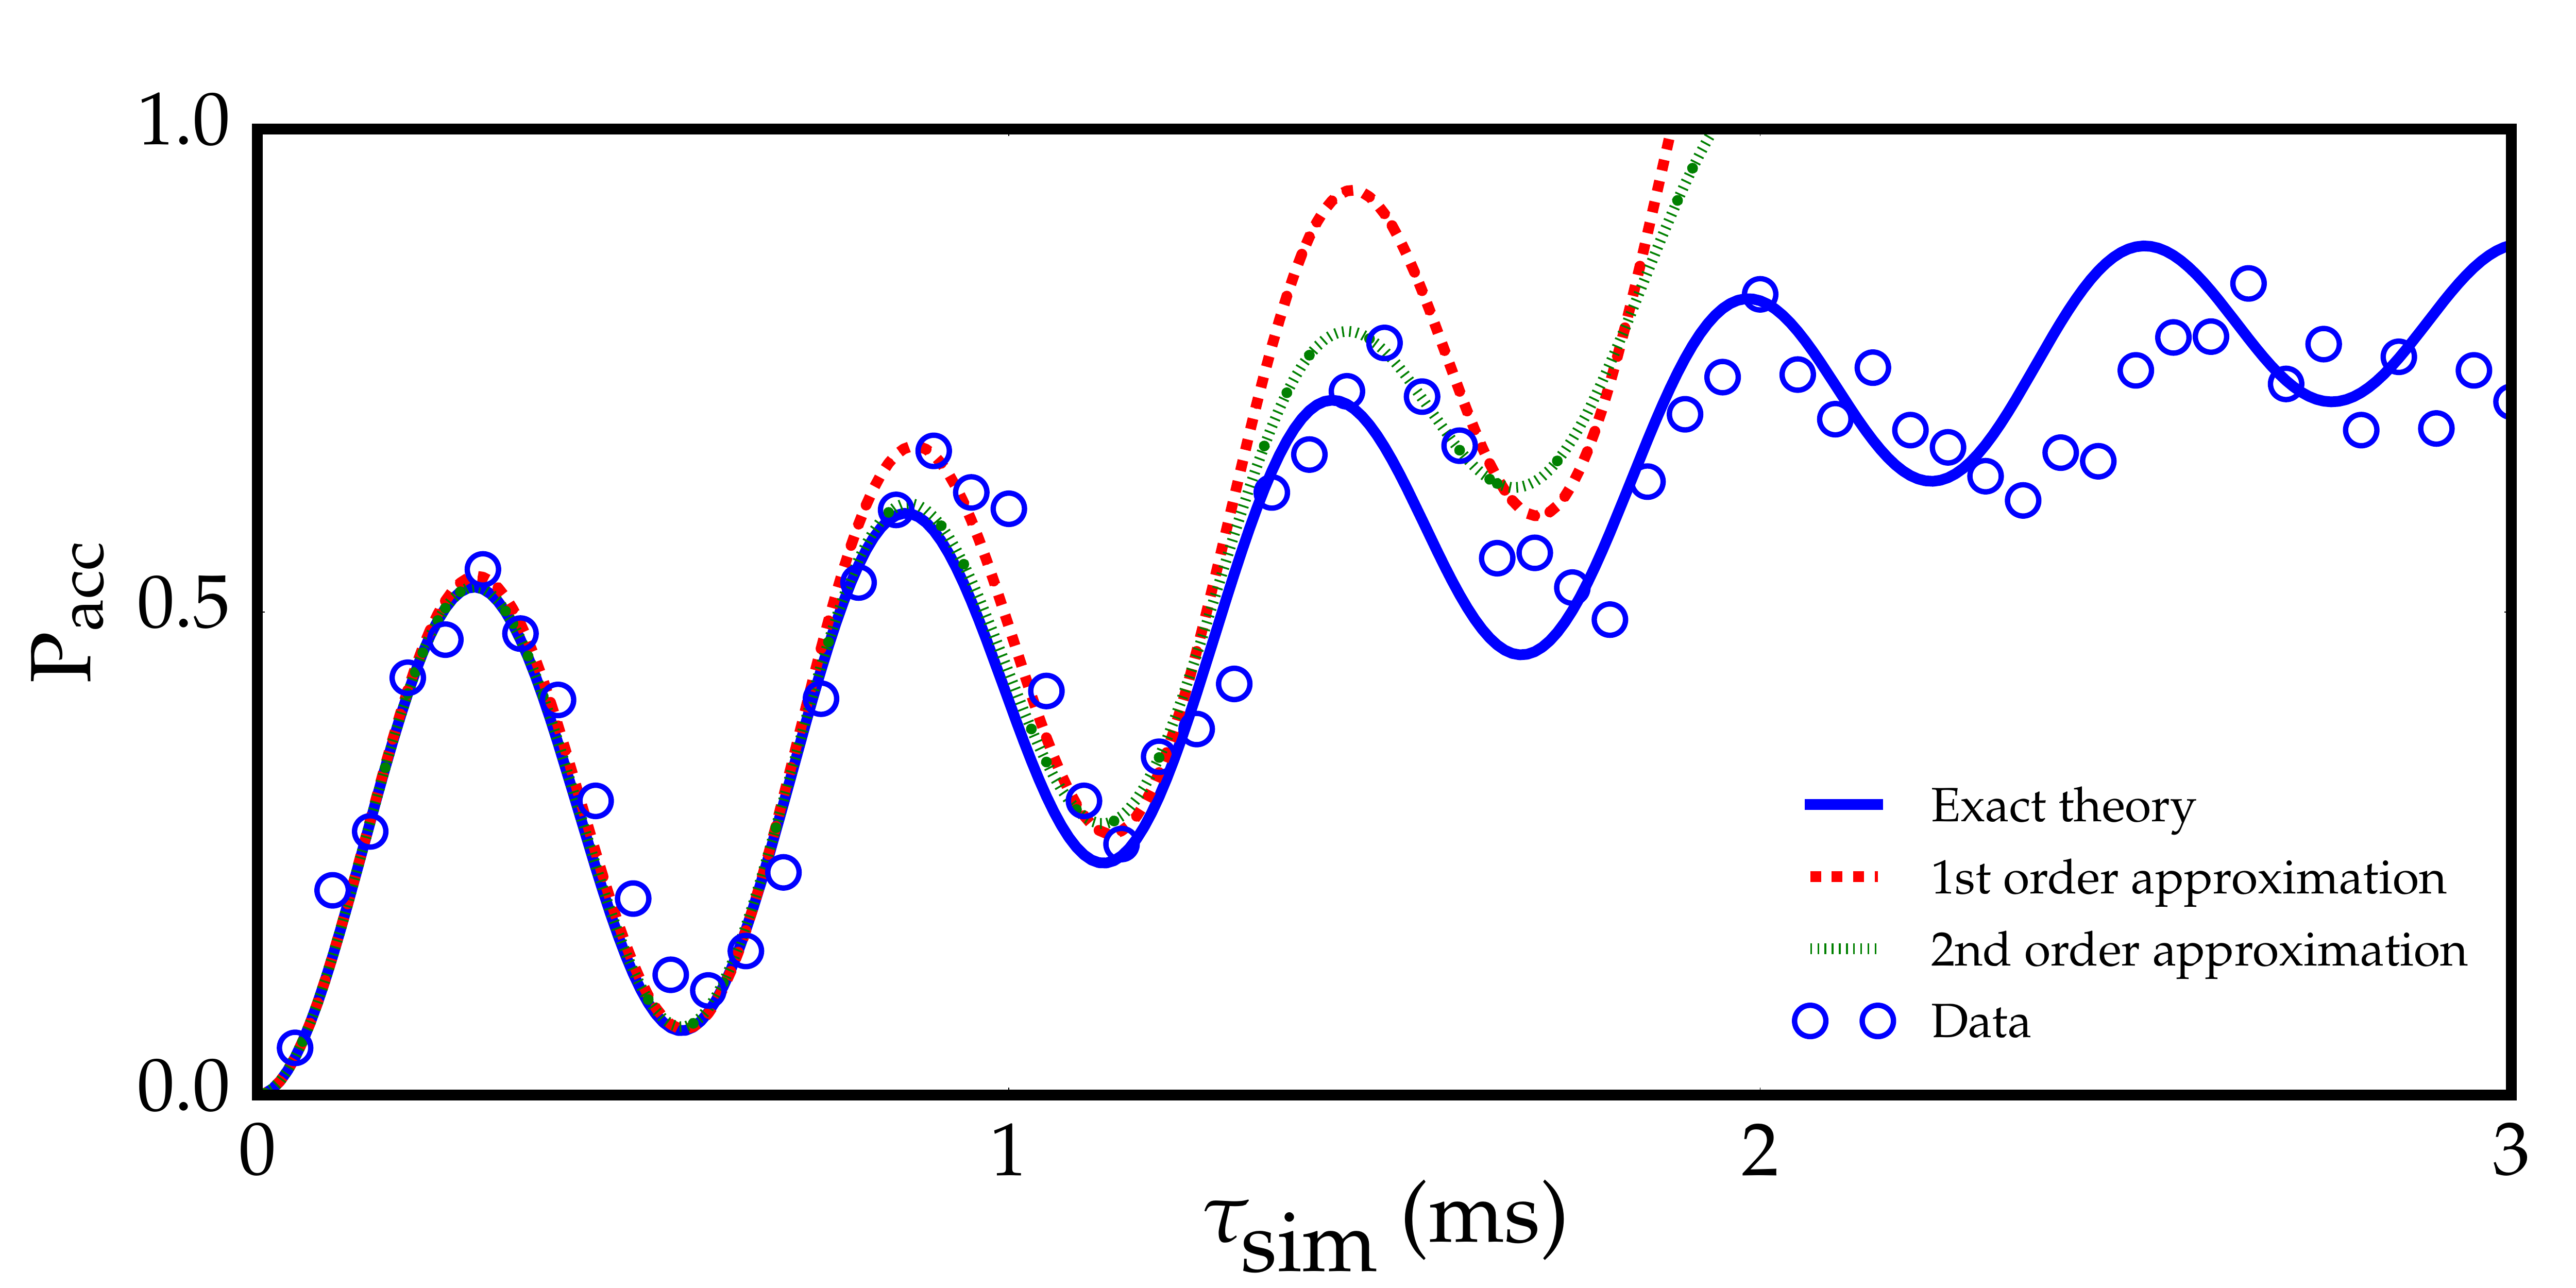}};
\node[inner sep=0pt] (trap) at (7.5,  0.0) {\includegraphics[width=0.45\textwidth]{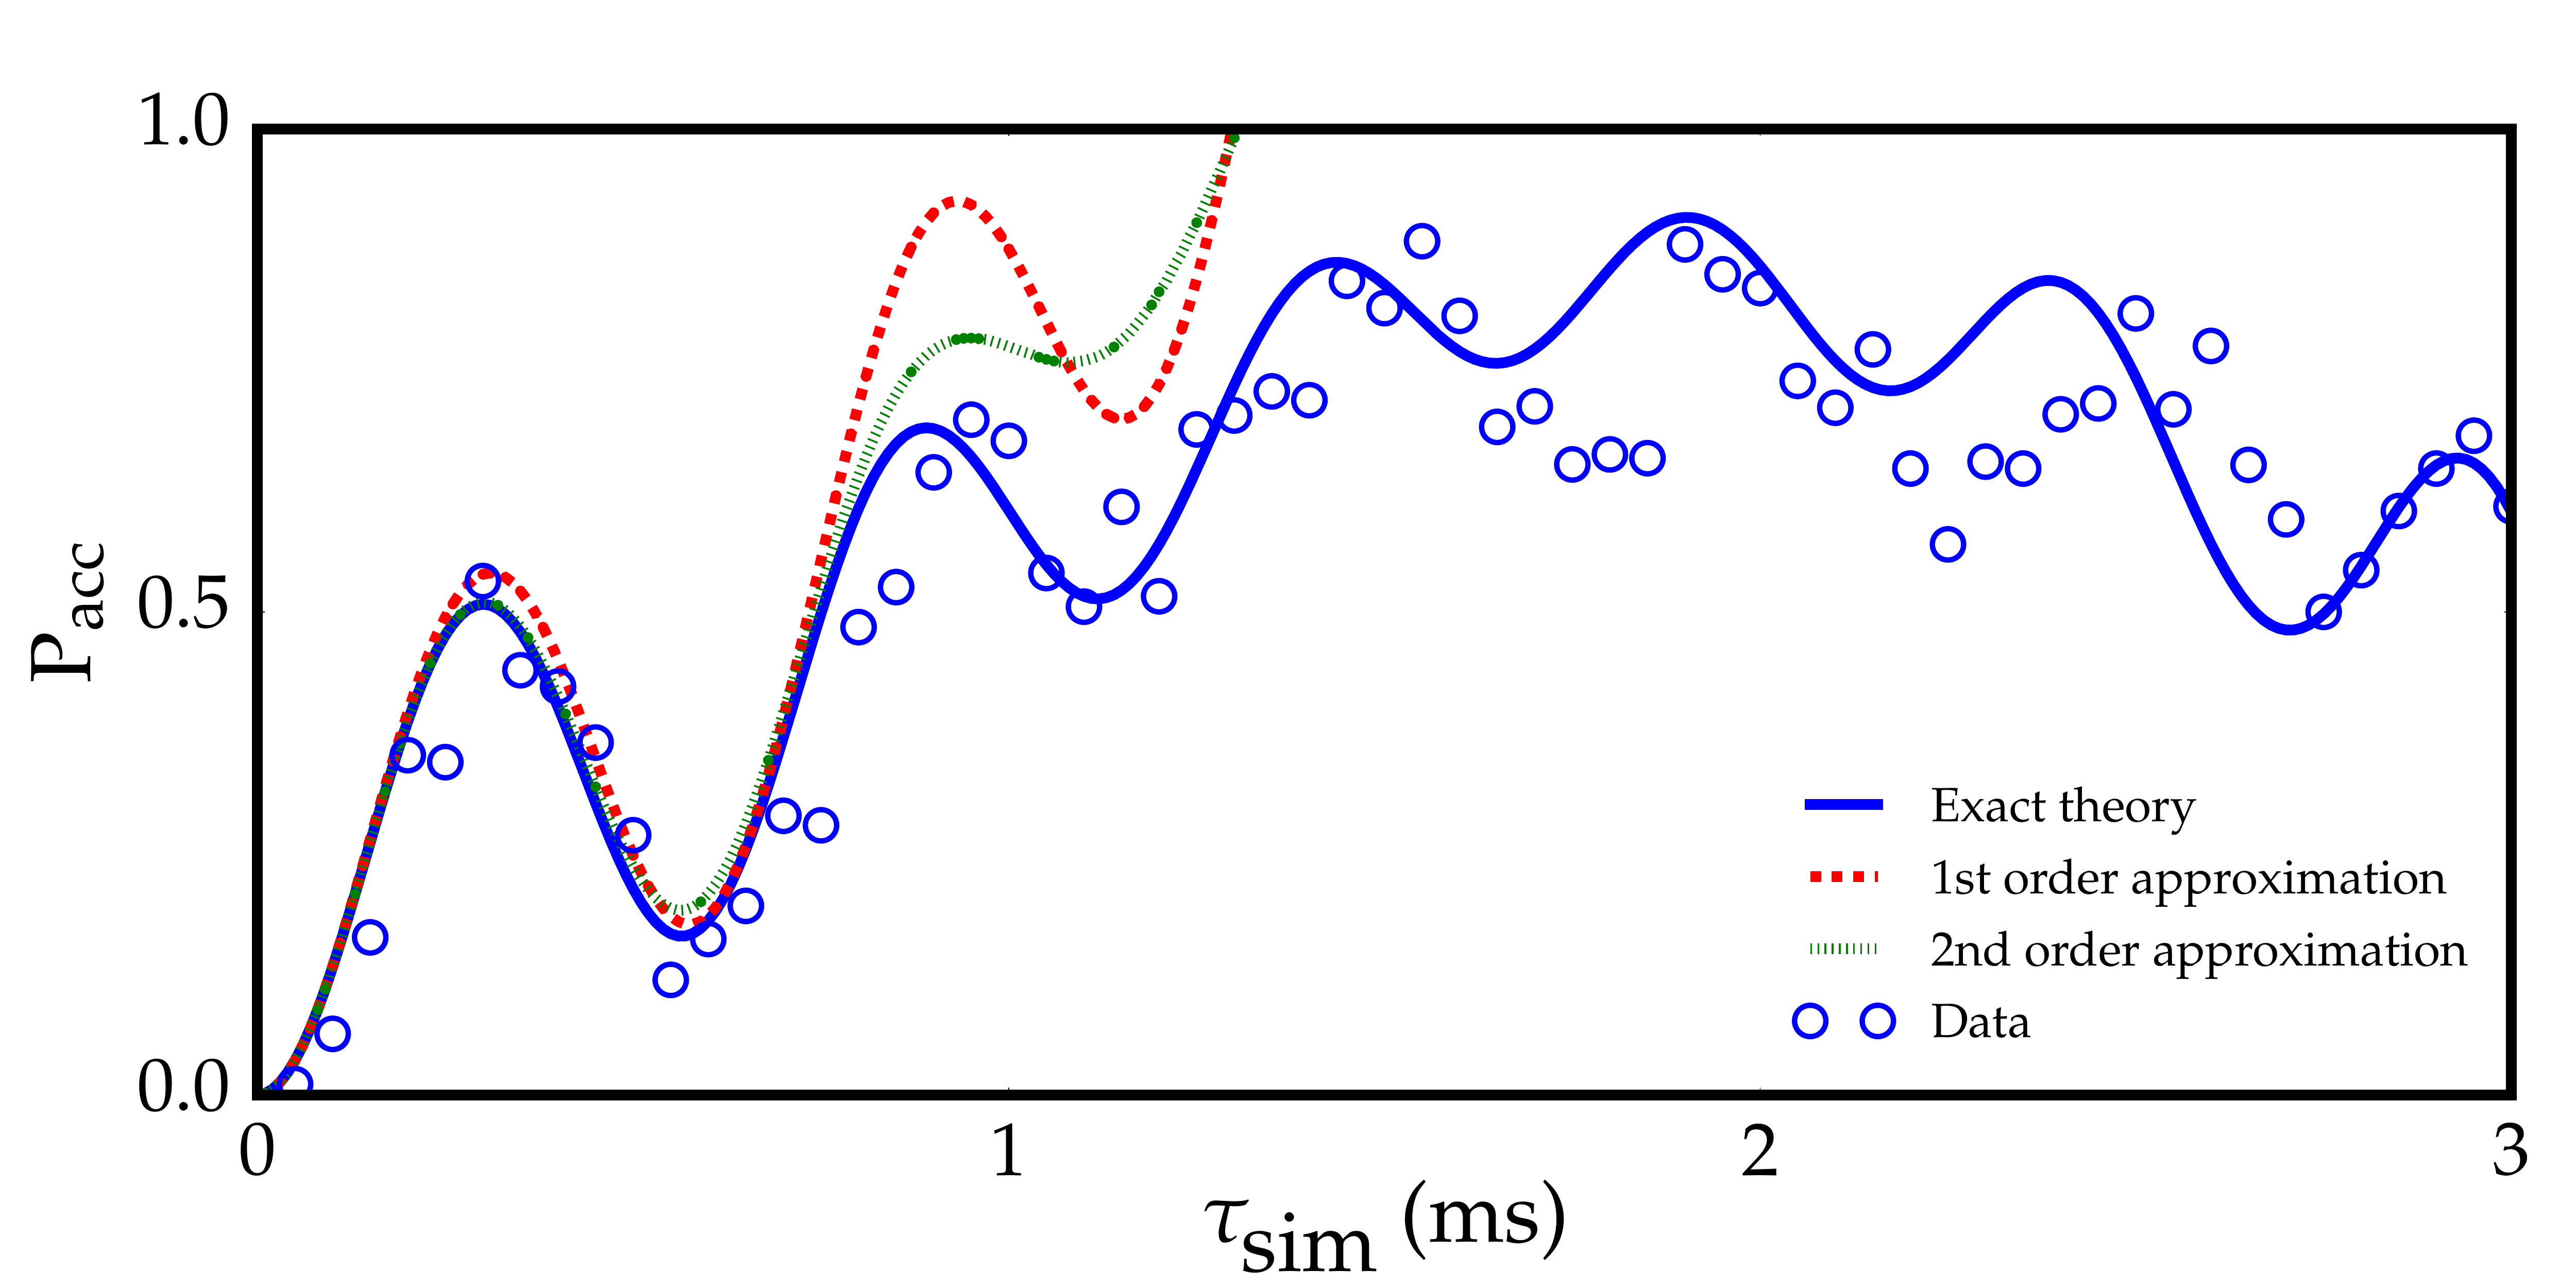}};
\node[inner sep=0pt] (trap) at (-1.0, -4.0) {\includegraphics[width=0.45\textwidth]{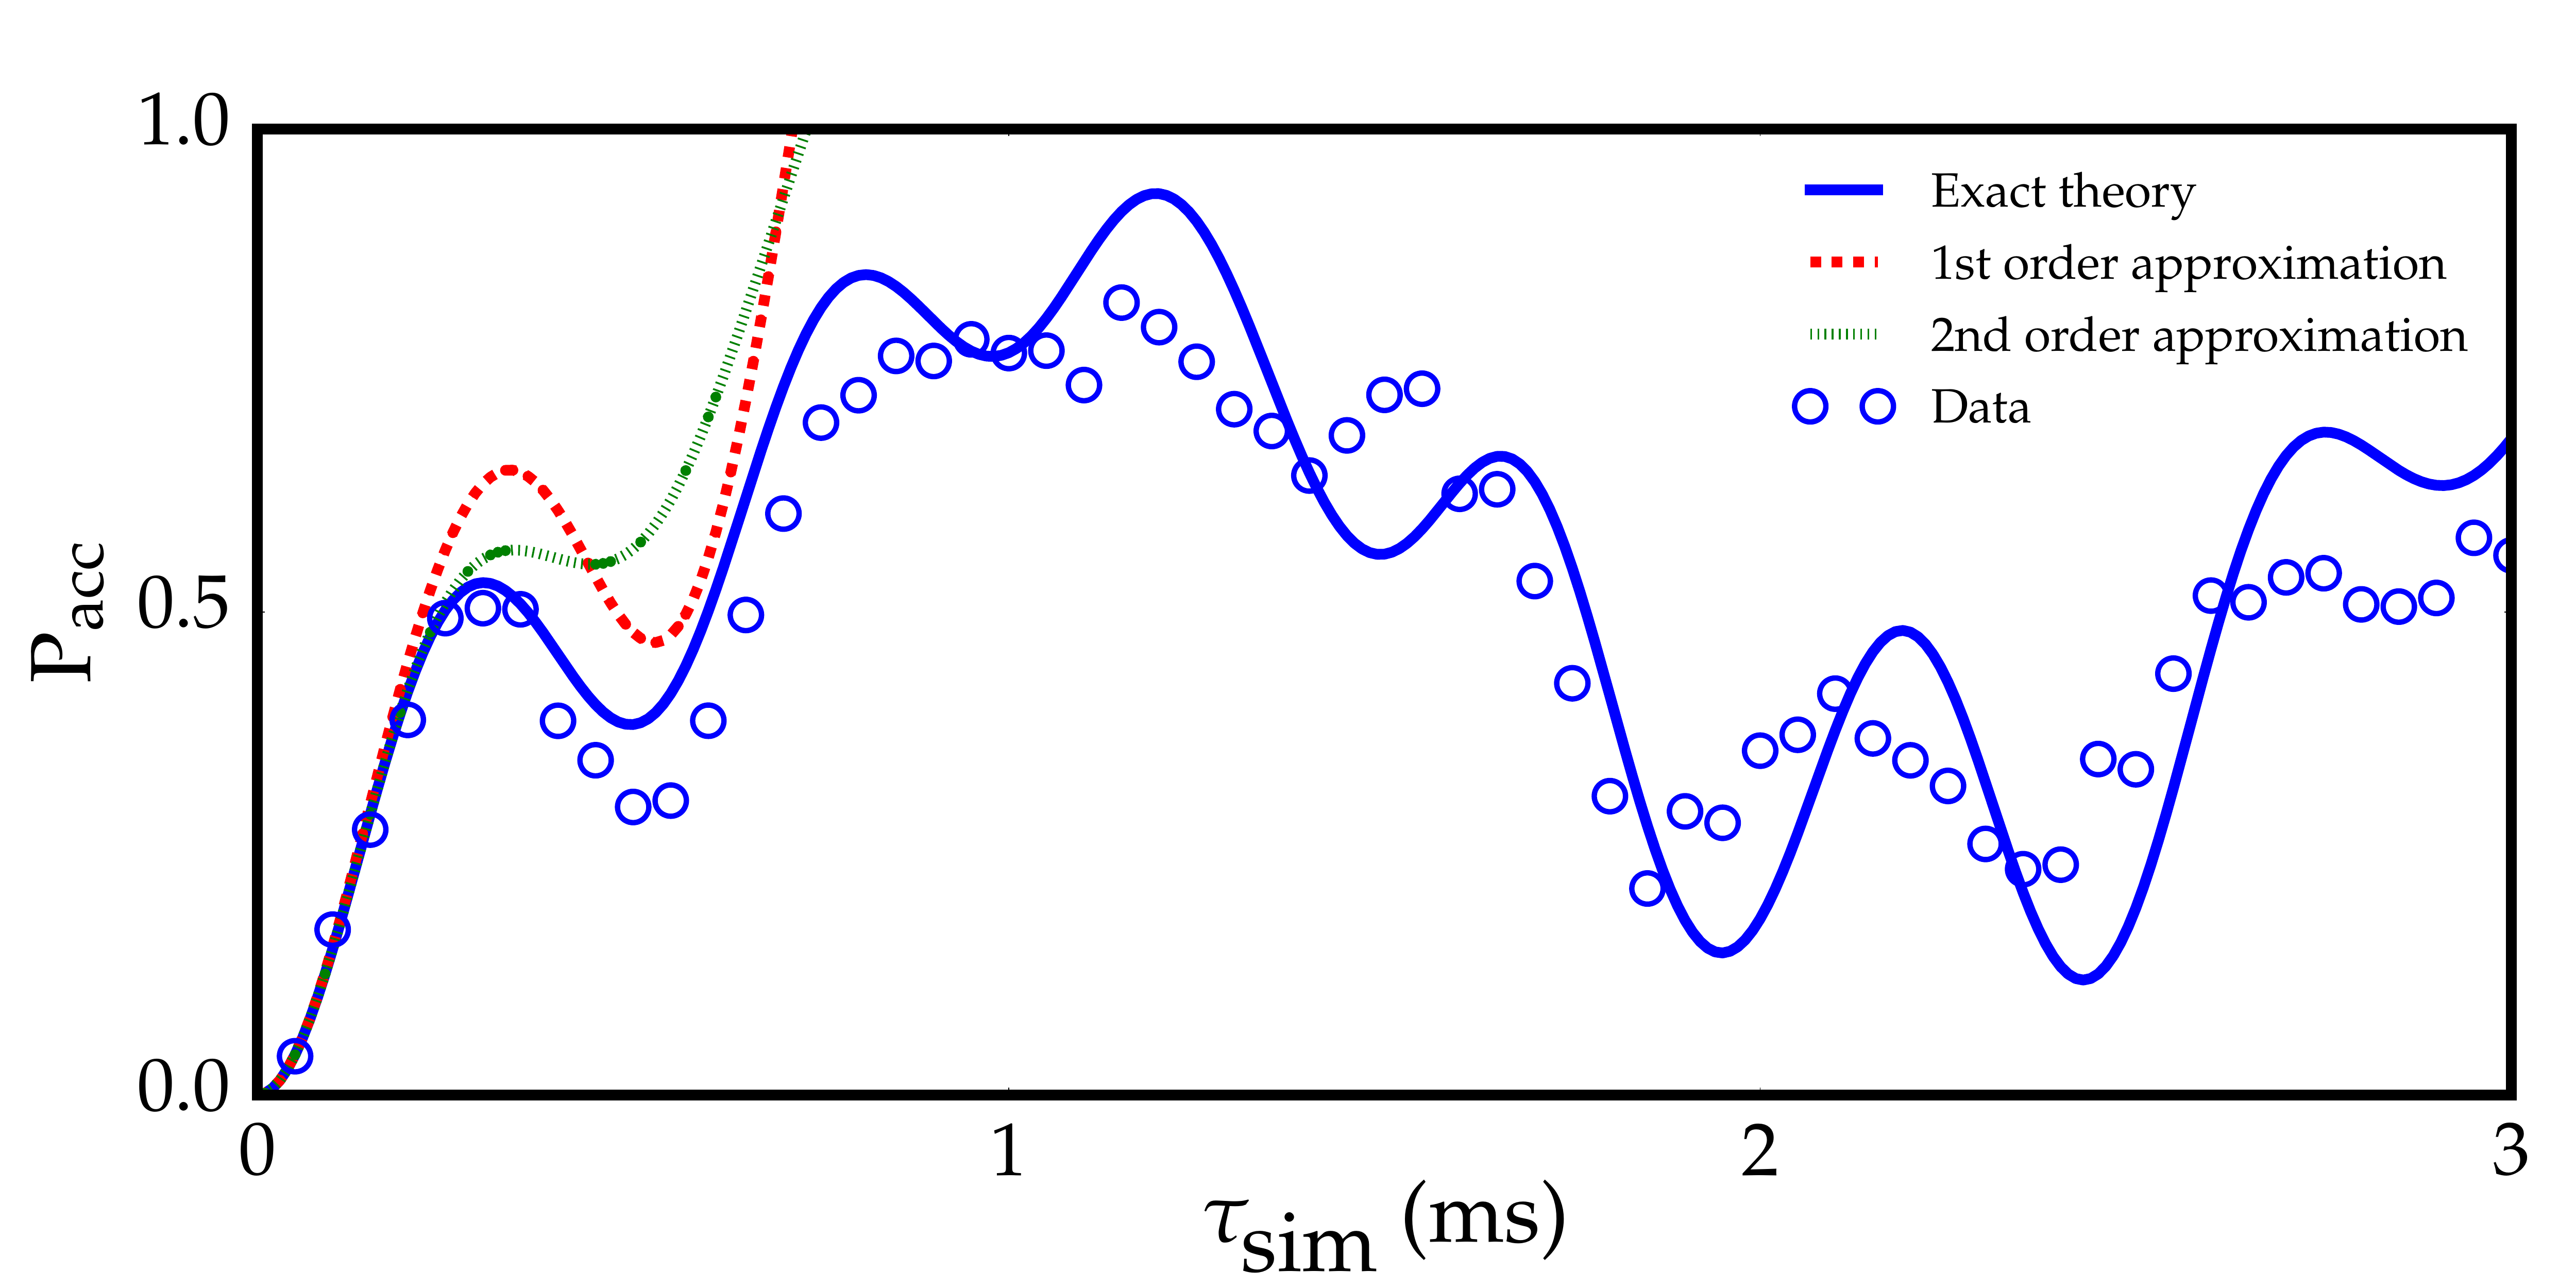}};

%\draw[draw, color = black, line width = 1pt, rounded corners, rounded corners = 3pt, scale = 1.0] (-7.4,-2.0) rectangle (1.4,2.25) {};

%\draw [line width = 1pt] (-3-0.2, -2.0) -- (-3-0.2, 2.25) {};

%\node at (-6.7, 1.55) {(a)};
%\node at (-6.7, -0.35) {(b)};
%\node at (0.9,  1.15) {(c)};

\end{tikzpicture}

\end{document}
